# Supplementary material for: Network Reconnaissance and Vulnerability Excavation of Secure DDS Systems
Source: arXiv:1908.05310 source file (2019-08-14)
Supplement: Supplementary file 2 [file appendix.tex]

\section{Appendix}
\label{par:appendix}

\input{figs/snippets/a_perm.tex}
\input{figs/snippets/b_perm.tex}

\input{figs/algorithms/dds_security_plugin.tex}
